# Supplementary material for: Optical Thouless conductance and level-spacing statistics in two-dimensional Anderson localizing systems
Source: arXiv:1910.14451 source file (2019-10-31)
Supplement: Supplementary file 1 [file Supplementary.pdf]

# Supplementary Information for

# Optical Thouless conductance and level-spacing statistics in two-dimensional Anderson-localizing systems

**Section.S1: Amorphous disorder**

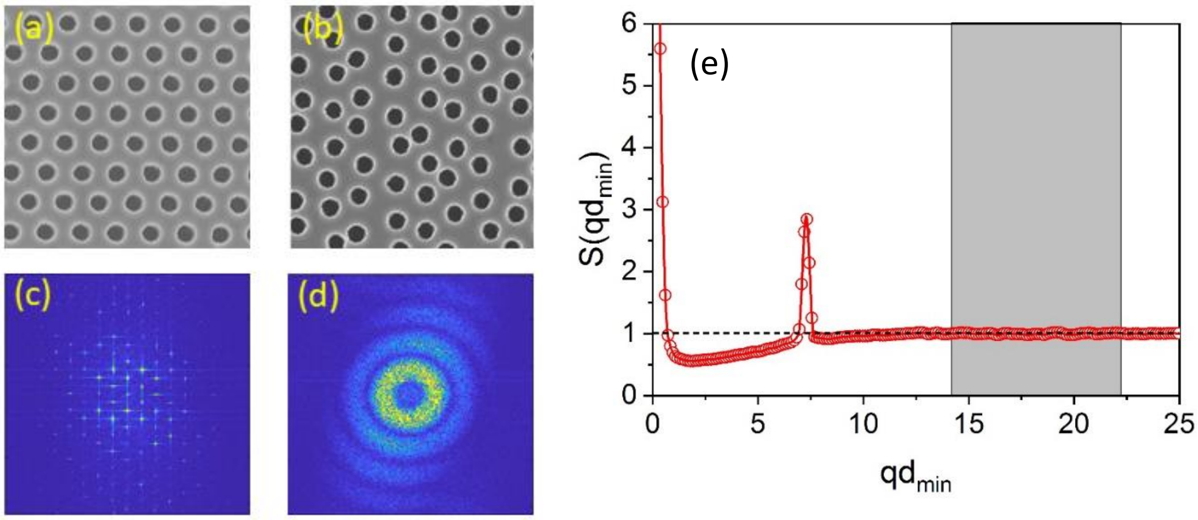


**Fig.S1:** SEM images of sections of the (a) periodic and (b) amorphous disordered samples. Fourier transforms of the (c) periodic and (d) amorphous sample images. (e) Structure factor of the disorder as a function of wave vector q. Grey box indicates the wavelength range of experiments, where S(q) = 1 uniformly.

Figure S1 (a) and (b) show the SEM images of the periodic and disordered membranes. (c) is the Fourier transform of the image of periodic samples and clearly shows discrete points (triangular lattice) in the Fourier space. (d) is the Fourier transform of disordered sample and shows a diffuse continuous distribution, owing to the fact that the periodicity is totally lost and the sample is amorphous. Figure S1 (e) shows the configurationally-averaged Structure factor for the disorder used in the samples, computed using the technique used in Ref 25 of the main manuscript. In the wavelength range used in the experiments (demarcated by the grey box), the S(q) is uniformly 1. This indicates that the disorder is uncorrelated, and our experimental observations arise from classical Anderson localization.

**Section.S2: Anderson-localized modes.**

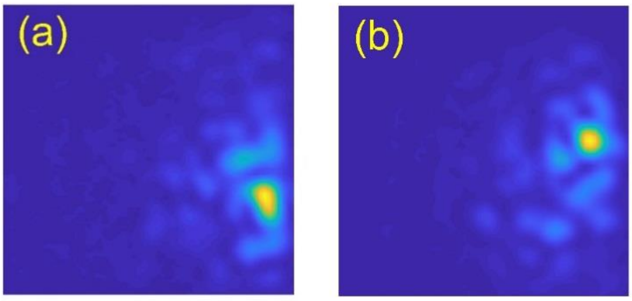


**Fig.S3:** (a), (b) Two representative localized mode profiles in two different configurations

Figure S2 shows two measured Anderson-localized mode profiles in two different configurations. The corresponding wavelengths are marked in Fig S5 in this document.

**Section.S3: Conductance '$g$' from Intensity Distribution**

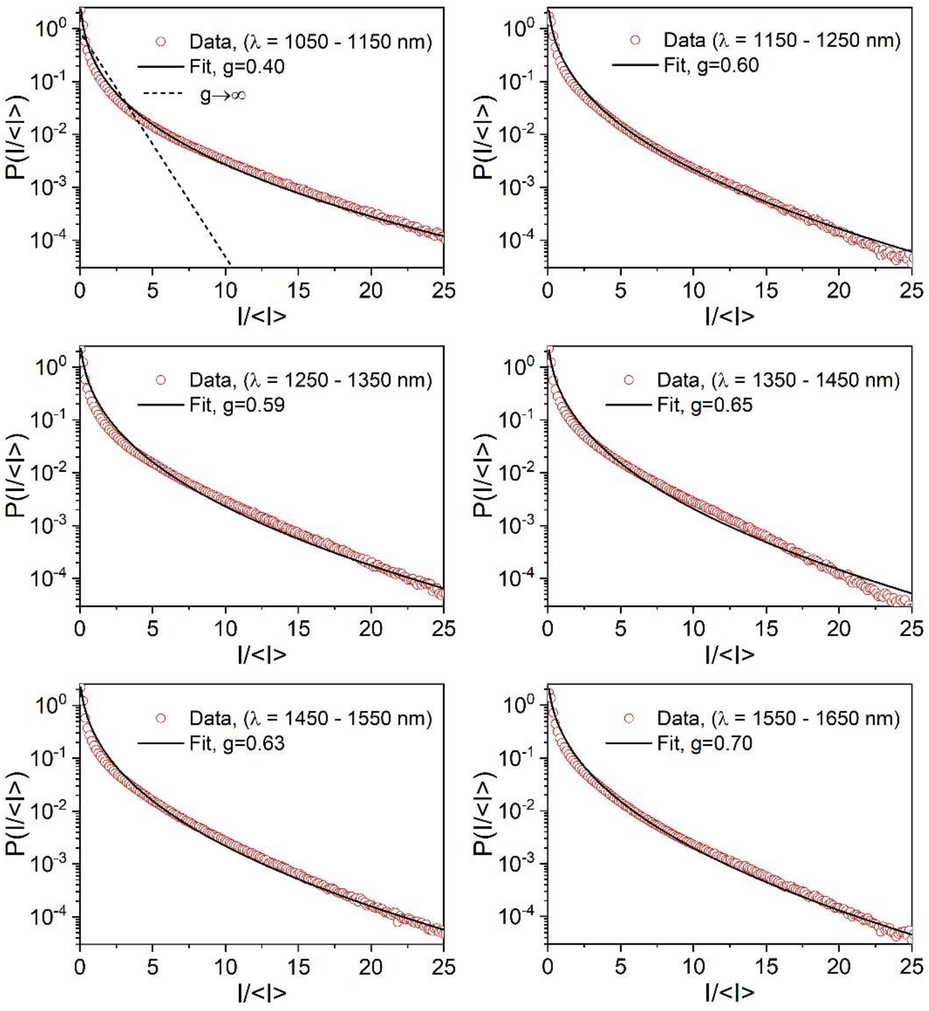


**Fig.S3:** Intensity statistics of the localized modes. Red circles are data and the black solid line is fit to the data. Dashed line shows the Rayleigh distribution.

Figure S3 shows the normalized intensity statistics of the Anderson-localized modes. The red circles are the data which shows a long-tailed behaviour as predicted for localized modes[R1, R2]. The black solid line is the theoretical fit. The black dashed line in the first sub-plot is the Rayleigh distribution which holds for diffusive modes with $g \rightarrow \infty$.

The wavelength range for each calculation was of 100 nm, to ensure sufficiently large ensemble for the averaging. In comparison, the Thouless conductance in the main paper was averaged over 50 nm.

**Section.S4: Loss length characterization.**

Figure S4 shows the loss length arising from the scattering loss. The inset shows the image of the configurationally-averaged intensity over 20 configurations in the periodic samples at

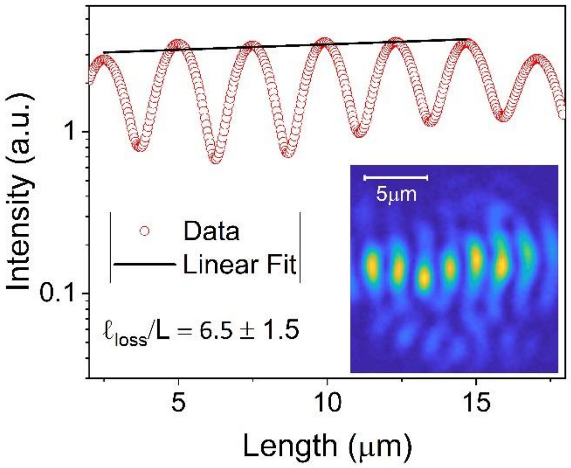


**Fig.S4:** Decaying intensity profile in the periodic structure. Black line is a linear fit to the data.

a particular wavelength in the passband range. Multiple configurations were created to account for the inherent disorder. Light is input from the right edge. The wavefronts of the superposition of forward and backward Bloch modes are seen in the image. In the main plot, the red circles depict the cross-section (along the propagation direction) of the intensity distribution. The black line is the fit to the peaks of the oscillating profile, and yield a loss length $\ell_{loss}/L = 6.5 \pm 1.5$. Similar analysis was carried out for other wavelengths, and yielded a loss length much larger than L.

**Section.S5: Intensity spectrum**

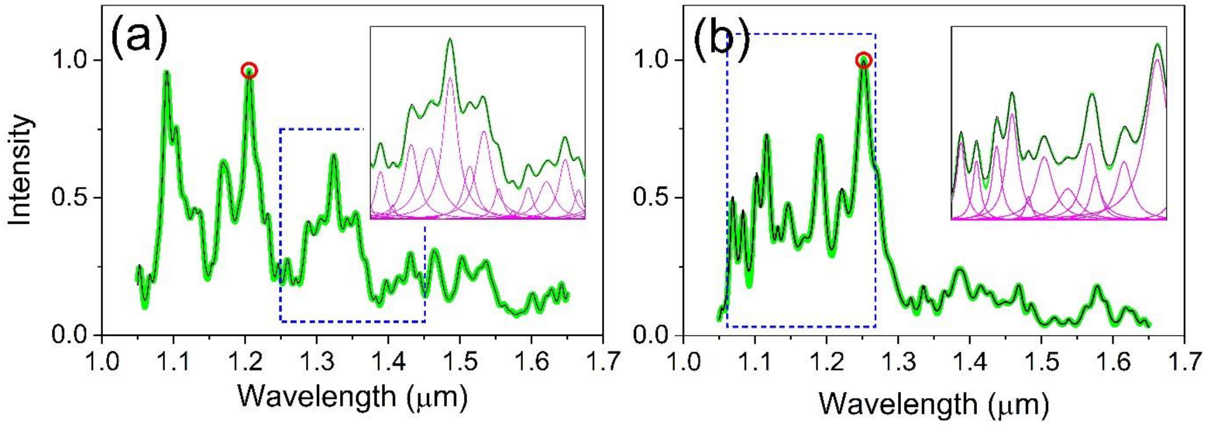


**Fig S5:** (a), (b) Two representative intensity spectra in two different configurations. The boxed areas are emphasized in the insets with the underlying Lorentzians explicitly shown.

Figure S5 shows two different intensity spectra for two configurations. The insets show the boxed area with the contribution Lorentzians. The red circles are the marked wavelengths where the mode profiles are shown in Fig.S2 in this document.

**References:**

[R1] M. C. W. van Rossum, and T. M. Nieuwenhuizen, Multiple scattering of classical waves: 428 microscopy, mesoscopy, and diffusion, Rev. Mod. Phys. 71, 313 (1999).

[R2] P. D. García, S. Stobbe, I. Söllner, and P. Lodahl, Nonuniversal Intensity Correlations in a Two-Dimensional Anderson-Localizing Random Medium, Phys. Rev. Lett. 109, 253902, (2012).
